# Supplementary material for: Range Description of a Conical Radon Transform
Source: arXiv:2110.11212 source file (2023-04-25)
Supplement: Supplementary file 1 [file Appendices.tex]

\begin{appendices}

\phantomsection

\section{Fourier Analysis Conventions and Properties} \label{cha: Appendix_Fourier}

The following sections detail the conventions used for the Fourier transform, as well as several important identities and theorems used throughout this dissertation.

\subsection{Fourier Transform} \label{sec: Fourier_Transform}
The Fourier transform of a function $f:\mathbb{R}^n \rightarrow \mathbb{R}$ is denoted $\hat{f}$ and defined as follows:
\begin{equation} \label{eq: Fourier_Transform}
    \hat{f}(\boldsymbol \omega) = \int_{\mathbb{R}^n} f(x) e^{-i \boldsymbol \omega \cdot \boldsymbol x} d \boldsymbol x.
\end{equation}
$\boldsymbol x$ and $\boldsymbol \omega$ are said to be \emph{dual variables}, and in general $\boldsymbol \omega \in \mathbb{C}^n$ when the above integral exists.

The corresponding inversion formula is given by
\begin{equation} \label{eq: Inverse_Fourier_Transform}
    f(\boldsymbol x) = \frac{1}{(2 \pi)^n} \int_{\mathbb{R}^n} \hat{f}( \boldsymbol \omega) e^{i \boldsymbol \omega \cdot \boldsymbol x} d \boldsymbol \omega.
\end{equation}

Identities such as the Fourier transforms of special functions, and composition of the Fourier transform and operators such as e.g. differentiation are easily derived and widely available, differing only by a constant depending on how the Fourier transform is defined. Rather than repeating such identities here, the reader is urged to refer to a text on Fourier analysis such as \cite{Strichartz}.

\subsection{Distributions and Test Functions} \label{sec: Distributions}
An important tool in the study of Fourier Analysis is the space of \emph{test functions}
\begin{equation}
    \mathcal{D}(\mathbb{R}^n) = C_{0}^{\infty}(\mathbb{R}^n)
\end{equation}
equipped with the family of seminorms
\begin{equation} \label{eq: seminorms}
    ||\psi||_{K,n} = \sup_{|\alpha| \leq n} \sup_{\boldsymbol x \in K} |\partial^{\alpha} \psi(\boldsymbol x)|
\end{equation}
where $\alpha$ is a multiindex, $n \in \mathbb{N}$ and $K$ ranges over all compact subsets of $\mathbb{R}^n$. Under these constraints, $D(\mathbb{R}^n$ is a locally convex topological vector space, with topology induced by the family of seminorms (\ref{eq: seminorms}). The continuous dual $D'(\mathbb{R}^n)$ is the space of continuous linear functionals $T:D(\mathbb{R}^n) \rightarrow \mathbb{R}$, and is known as the space of \emph{distributions}. Many distributions can be written in the form:
\begin{equation}
    T(\psi) = \int_{\mathbb{R}^n} f(\boldsymbol x) \psi(\boldsymbol x) d \boldsymbol x
\end{equation}
for some function $f$. For this reason, the action of a distribution on a test function is written
\begin{equation}
    T(\psi)=<T,\psi>
\end{equation}

We can consider a broader class of test functions, namely \emph{Schwartz functions}:
\begin{equation}
    \mathcal{S}(\mathbb{R}^n) =\{f \in C^{\infty} (\mathbb{R}^n): \forall \alpha, \beta \in \mathbb{N}^n,||f||_{\alpha,\beta} < \infty\}
\end{equation}
where the family of seminorms $||\cdot||_{\alpha,\beta}$ is defined by:
\begin{equation}
    ||f||_{\alpha,\beta} = \sup_{\boldsymbol x \in \mathbb{R}^n} |\boldsymbol x^{\alpha}\partial^{\beta} f (\boldsymbol x)|.
\end{equation}
An important fact relating the space of test functions and the space of Schwartz functions is that the space of test functions is dense in the space of Schwartz functions. The dual space $S'(\mathbb{R}^n)$ is known as the space of \emph{tempered distributions}. Because the space of test functions is dense in the space of Schwartz functions, tempered distributions can be expressed as the limit of a sequence of distributions. Another important fact about the space of Schwartz functions is that the Fourier transform is an isometry on the space of Schwartz functions.

In general distributions may be much more pathological than a function, for instance, the well known Dirac delta distribution $\delta(\boldsymbol x)$, defined by $<\delta,\psi>=\psi(0)$ cannot be represented with a function. 

Nonetheless, we can define the Fourier transform of any tempered distribution as follows:
\begin{equation} \label{eq: Fourier_Transform_Distribution}
    <\hat{T},\psi> = <T,\hat{\psi}>.
\end{equation}
That is, $\hat{T}$ is the unique tempered distribution whose action on $\psi$ is the same as the action of $T$ on the Fourier transform of $\psi$.

The theory of distributions is rich and powerful, and an extensive discussion is beyond the scope of this appendix, but the interested reader is referred to \cite{Strichartz} for an excellent introduction to the topic.

\subsection{Paley--Wiener Theorems} \label{sec: PW_Theorems}
A fundamental set of theorems in the study of Fourier analysis are the Paley--Wiener type theorems, which relate the decay of distributions to the smoothness and growth of their Fourier transform. We will state without proof a few of the Paley--Wiener type Theorems used in this dissertation.

\begin{theorem}[P.W. 1]
    Let $f \in C_0^{\infty}(B_R(0))$, then $\hat{f}$ is an entire function of exponential type $R$ (that is, there is a constant $C$ so that $|\hat{f}(\boldsymbol \omega)| \leq Ce^{R|\boldsymbol \omega|}$) and $\hat{f}$ is rapidly decreasing (that is, $|\hat{f}(\boldsymbol \omega)| \leq C_N(1+|\boldsymbol \omega|)^{-N}$ for all $N$). Conversely, if $g$ is a rapidly decreasing entire function of exponential type $R$, then $g=\hat{f}$ for some $f \in C_0^{\infty}(B_R(0))$ \cite{Strichartz}.
\end{theorem}

\begin{theorem}[P.W. 2]
    Let $f$ be a distribution supported on  $B_R(0)$, then $\hat{f}$ is an entire function satisfying the growth estimate
    \begin{equation*}
        |\hat{f}(\boldsymbol \omega| \leq C(1+|\boldsymbol \omega|)^N e^{R |\boldsymbol \omega|}
    \end{equation*}
    for some $C$ and $N$. Conversely, if $g$ is an entire function satisfying the above growth estimate, then $g=\hat{f}$ for some distribution $f$ supported on $B_R(0)$ \cite{Strichartz}.
\end{theorem}

\begin{theorem}[P.W. 3] \label{thm: PW3}
    Let $f$ be a tempered distribution supported on the half space $x_n > 0$, then $\hat{f}$ can be analytically continued to the the set $\mathbb{R}^{n-1} \times \mathbb{H}_-$, where $\mathbb{H}_-=\{z \in \mathbb{C}:\Im(z)<0\}$. Moreover, 
    \begin{equation*}
        \hat{f}(\boldsymbol \omega) = \lim_{\eta \rightarrow 0} \hat{f}(\omega_1,\omega_2,...,\omega_{n-1},\omega_n + i \eta) \qquad \boldsymbol \omega \in \mathbb{R}^n
    \end{equation*}
    in the sense of distribution. Conversely, if $g$ is an analytic function on $\mathbb{R}^{n-1} \times \mathbb{H}_-$, there is a unique tempered distribution $f$ supported on the half-space $x_n > 0$ such that
    \begin{equation*}
        \hat{f} (\boldsymbol \omega) = \lim_{\eta \rightarrow 0} g(\omega_1,\omega_2,...,\omega_{n-1},\omega_n + i \eta) \qquad \boldsymbol \omega \in \mathbb{R}^n
    \end{equation*}
    in the sense of distribution \cite{Bremmerman, Strichartz, Sharyn1999}.
\end{theorem}
\end{appendices}
